# Supplementary material for: Revisiting Robustness in Priced Timed Games
Source: arXiv:1507.05787 source file (2015-07-21)
Supplement: Supplementary file 1 [file robust-appendix.tex]

%\section{Detailed Description of Some Modules Used in the Undecidability Result}
%
%\input{./figs/mchoice.tex}
%\paragraph{mChoice module}:
%Like the choice module, in the mChoice module also the value of clocks $x_1$, $z$ and $x_2$ are increased
%by 3 while clocks $y_1$ and $y_2$ have value 0 on exit.
%
%\paragraph{Restore modules}:
%The $Restore_{Inc}^{C_2C_1}$ module can be obtained from $Restore_{Inc}^{C_1C_2}$ module by
%replacing all the occurrences of clock $x_1$ with clock $z$ and
%replacing all the occurrences of clock $z$ with clock $x_1$.
%$Restore_{Dec}^{C_2C_1}$ can also be obtained from
%$Restore_{Dec}^{C_1C_2}$ in the same way.
%The edge from location $C$ to location $D$ forces controller
%to take the loop at location $C$ only once.
%Corresponding to $Restore_{Inc}^{C_1C_2}$,
%the delays at locations $A$, $C$ and $D$ are
%$1-\frac{1}{2^i}-\varepsilon_1$,
%$\frac{1}{2^i}+\varepsilon_1 - \frac{1}{2^j}-\varepsilon_2$
%and $\frac{1}{2^j}+\varepsilon_2$ respectively,
%while the delays at locations $B$ and $E$ are 0.
%The value of clock $z$ at the entry of the $Restore_{Dec}^{C_1C_2}$
%and $Restore_{Dec}^{C_2C_1}$ is $5+\frac{1}{2^j}+\varepsilon_2$
%and the the clock values at the exit are as
%$Restore_{Inc}^{C_1C_2}$ and $Restore_{Inc}^{C_2C_1}$ modules.
%
%\paragraph{Decrement $C_1$ module}:
